# Supplementary material for: The N$^3$LO Twist-2 Matching of Linearly Polarized Gluon TMDs
Source: arXiv:2509.01703 ancillary file (2026-04-04)
Supplement: Supplementary file 1 [file readme.pdf]

# Ancillary Files for “The N<sup>3</sup>LO Twist-2 Matching of Linearly Polarized Gluon TMDs”

Yu Jiao Zhu<sup>1,\*</sup>

<sup>1</sup>*Zhejiang Institute of Modern Physics, Department of Physics, Zhejiang University, Hangzhou, 310027, China*

In this note we explain the definitions and conventions for the ancillary files associated with the arXiv submission of “The N<sup>3</sup>LO Twist-2 Matching of Linearly Polarized Gluon TMDs”.

## TMD BEAM FUNCTION

In the MATHEMATICA file `lBeam.m` and `lBeamN.m`, we provide coefficient functions for the transverse-momentum-dependent (TMD) beam function for the linearly polarized gluon distributions. They correspond to Eqs. (3.4) in the paper, with

$$\text{lBeam}["\text{gi}"] = \text{as} \mathcal{I}'_{gi}{}^{(1)} + \text{as}^2 \mathcal{I}'_{gi}{}^{(2)} + \text{as}^3 \mathcal{I}'_{gi}{}^{(3)}, \quad (1)$$

where “as” stands for  $\frac{\alpha_s(\mu)}{4\pi}$ , and  $\mathbf{i} = \mathbf{q}$ ,  $\mathbf{g}$  stands for the target parton with quark  $q$  or gluon  $g$ . For example, after loading the file, type in `lBeam["gq"]` will return the result for  $\mathcal{I}'_{gq}(x, b_\perp, \mu, \nu)$ .

We use the following definitions and conventions in the file:

$$L_p = L_\perp = \ln(|b_\perp|^2/\mu^2/b_0^2), \quad L_Q = L_Q = 2 \ln(Q/\nu), \quad (2)$$

where  $Q = xP^+$  is the momentum flow into the hard scattering.

## TMD PARTON DISTRIBUTION FUNCTION

The MATHEMATICA file `lPDF.m` and `lPDFN.m` give the results for the rapidity-regulator-independent linearly polarized gluon TMD PDFs,

$$h_{1,gi}^\perp(x, b_\perp, \mu) = \mathcal{I}'_{gi}(x, b_\perp, \mu, \nu) \sqrt{\mathcal{S}(b_\perp, \mu, \nu)}. \quad (3)$$

They have the same naming convention as the in file `lBeam.m`, with the introduction of the Collins-Soper scale logarithm

$$L_h = L_\nu + L_Q = \ln(Q^2/\mu^2), \quad (4)$$

in

$$\text{lPDF}["\text{gi}"] = \text{as} h_{1,gi}^{\perp,(1)} + \text{as}^2 h_{1,gi}^{\perp,(2)} + \text{as}^3 h_{1,gi}^{\perp,(3)}. \quad (5)$$

$L_\nu$  is the rapidity logarithm in the TMD soft function

$$L_\nu = L_\nu = \ln(\nu^2/\mu^2). \quad (6)$$

## THE TIME-LIKE TMD COEFFICIENT FUNCTIONS

In the MATHEMATICA file `lFrag.m` and `lFragN.m`, we provide time-like coefficient functions for the linearly polarized gluon TMD distributions. They correspond to

Eqs. (3.6) in the paper, with

$$\text{lFrag}["\text{ig}"] = \text{as} \mathcal{C}'_{ig}{}^{(1)} + \text{as}^2 \mathcal{C}'_{ig}{}^{(2)} + \text{as}^3 \mathcal{C}'_{ig}{}^{(3)}, \quad (7)$$

$\mathbf{i} = \mathbf{q}$ ,  $\mathbf{g}$  stands for  $g$  decay into quark  $q$ , gluon  $g$ . For example, after loading the file, type in `lFrag["qg"]` will return the result for  $\mathcal{C}'_{qg}(z, b_\perp/z, \mu, \nu)$ . Our results for the TMD fragmentation functions are in the hadron frame, where the detected hadron has zero transverse momentum.

We use the following definitions and conventions in the file:

$$L_p = L_\perp = \ln(|b_\perp|^2/\mu^2/b_0^2), \quad L_Q = L_Q = 2 \ln(Q/\nu), \quad (8)$$

where  $Q = P^+/z$  is twice the energy of the fragmented parton.

## TMD FRAGMENTATION FUNCTION

The MATHEMATICA file `lFF.m` and `lFFN.m` give the results for the rapidity-regulator-independent TMDFFs for the linearly polarized gluon,

$$h_{1,ig}^{T\perp}(z, b_\perp/z, \mu) = \mathcal{C}'_{ig}(z, b_\perp/z, \mu, \nu) \sqrt{\mathcal{S}(b_\perp, \mu, \nu)}. \quad (9)$$

They have the same structure as the file `lFF.m`, with the introduction of the Collins-Soper scale logarithm

$$L_h = L_\nu + L_Q = \ln(Q^2/\mu^2), \quad (10)$$

in

$$\text{lFF}["\text{ig}"] = \text{as} h_{1,ig}^{T\perp,(1)} + \text{as}^2 h_{1,ig}^{T\perp,(2)} + \text{as}^3 h_{1,ig}^{T\perp,(3)}. \quad (11)$$

## RESUMMED TIME-LIKE COEFFICIENT FUNCTIONS

In the MATHEMATICA file `resummedFFsingles.m`, we provide the Mellin N-space results for the resummed time-like coefficient functions to order  $a_s^{15} = (\alpha_s/(4\pi))^{15}$ , where the expressions of the respective highest three terms in the Laurent expansions about  $\bar{N} = N - 1 = 0$  are given. The corresponding  $z$ -space results are obtained by inverse Mellin transformation, and according to our definition of the Mellin moments

$$\begin{aligned} M \left[ \frac{1}{z} \ln^k z \right] &\equiv \int_0^1 dz z^{N-1} \frac{1}{z} \ln^k z \\ &= \frac{(-1)^k k!}{(N-1)^{k+1}} = \frac{(-1)^k k!}{\bar{N}^{k+1}}, \end{aligned} \quad (12)$$

the inversion rule is simply given by

$$\overline{N}^k \rightarrow -\frac{(-1)^{-k}}{(-k-1)!} \ln^{-k-1} z, \quad \forall k < 0. \quad (13)$$

## SYMBOLS AND COLORS

For the color factors,

$$\begin{aligned} \mathbf{CF} &= C_F, \quad \mathbf{Nf} = N_f, \quad \mathbf{TF} = T_F, \quad \mathbf{CA} = C_A, \\ \frac{\mathbf{dabc2}}{\mathbf{nc}} &= \frac{d^{ABC} d_{ABC}}{N_c} = \frac{(N_c^2 - 1)(N_c^2 - 4)}{N_c^2}. \end{aligned} \quad (14)$$

`plusD[n,1-z]` is the conventional plus distribution

$$\text{plusD}[n,1-z] = \left( \frac{\ln^n(1-z)}{1-z} \right)_+. \quad (15)$$

Dirac delta function is represented by

$$\mathbf{delta}[1-z] = \delta(1-z).$$

Harmonic polylogarithms are represented by

$$\mathbf{H}[\mathbf{a1}, \mathbf{a2}, \dots, \mathbf{an}, z] = \text{HPL}[\{\mathbf{a1}, \mathbf{a2}, \dots, \mathbf{an}\}, z],$$

and `zeta[n]` is Riemann zeta value  $\zeta_n$ .

When referring to the linearly polarized gluon TMD distributions and fragmentation functions calculated in this paper, please kindly cite Refs. [1].

---

\* zhuyujiao@zju.edu.cn  
 [1] Y.J. Zhu, “The N<sup>3</sup>LO Twist-2 Matching of Linearly Polarized Gluon TMDs,” [arXiv:25??xxxx [hep-ph]].
